# Supplementary material for: Optimization for Neural Operators can Benefit from Width
Source: arXiv:2502.00705 source file (2025-02-02)
Supplement: Supplementary file 1 [file DeepONetNTK.tex]

\subsection{Optimization Guarantees for DeepONets: ReLU Activations}\label{subsec:ReLUProofs}
Recall the DeepONet predictor \eqref{eq:DeepONetPredictor}
\begin{equation}
    G_{\vtheta}\left(u^{(i)}\right)(y^{(i)}_j) 
    :=  
    \sum_{k=1}^K f_k \left(\vtheta_f; u^{(i)}\right) 
                 g_k\left(\vtheta_g; y^{(i)}_j\right)~.
    \label{eq:output_DeepONet_Appdx}
\end{equation}
In the analysis, it is useful to distinguish between the parameters up to the pre-final layer and the final layer, i.e. $\dim (\vtheta) = M_f + M_g + (m_f+m_g) K$, where $M_f$ and $M_g$ denote the number of parameters in the branch and trunk nets till the pre-final layer respectively and $m_f \cdot K$ and $m_g\cdot K$ are the number of weights in the last layer of the branch and trunk nets respectively. In essence we have $\dim (\vtheta_f) = M_f + m_f \cdot K$ and  $\dim (\vtheta_g) =  M_g + m_g \cdot K$. 
We note that it is sufficient to show positive definiteness of the above NTK at initialization. Once that has been established, standard approaches \citet{jacot2018neural,du2019gradient,Arora_Du_Neurips_2019,arora2019fine,allen-zhu_convergence_2019} allow one to show the geometric convergence of GD. In the sequel it proves useful to rewrite the branch and trunk net outputs as:
\begin{align}
f_k \left(\vtheta_f; u^{(i)}\right) = \sum_{h=1}^{m_f} w_{k,h}^{(f)} \bar{f}_h \left(\vtheta_{\bar{f}}; u^{(i)}\right) ~, \quad g_k \left(\vtheta_g; y^{(i)}_j \right) = \sum_{h'=1}^{m_g} w_{k,h'}^{(g)} \bar{g}_{h'} \left(\vtheta_{\bar{g}}; y^{(i)}_j \right)~, \quad \forall\; k\in [K],
\label{eq:fkone}
\end{align}
where $w_{k,h}^{(f)}, h \in [m_f]$ are the weights of the linear last layer of the branch net and $w_{k,h'}^{(g)}, h^{\prime} \in [m_g]$ are the weights of the linear last layer of the trunk net. Similarly, $\vtheta_{\bar{f}}$ and $\vtheta_{\bar{g}}$ are the parameters leading up to the pre-final layer in branch net with $m_f$ outputs $[\bar{f}_h, h \in [m_f]]$ and trunk net with $m_g$ outputs $[\bar{g}_{h'}, h' \in [m_g]]$ respectively. We will denote by $\vtheta_{f,k}$ all the parameters corresponding to $f_k$, i.e. $\vtheta_{f,k} := \{ w_{k,h}^{(f)}, h \in [m_f], \vtheta_{\bar{f}} \}$ which includes all the parameters needed for $f_k$ for each $k \in [K]$. Similarly we denote by $\vtheta_{g,k}$, all the parameters corresponding to $g_k$, i.e. $\vtheta_{g,k} := \{ w_{k,h'}^{(g)}, h' \in [m_g], \vtheta_{\bar{g}} \}$.

We can explicitly write the NTK for the DeepONet model, specifically entry corresponding to the inputs $\{u^{(i)}, y^{(i)}_j\}$ and $\{u^{(i')}, y^{(i')}_{j'}\}$ as:
% \abcomment{needs clean-up, use the vector perspective, avoid $\nabla_{\vtheta}$}
\begin{align}
    \begin{aligned}
        \left\langle  \nabla_{\vtheta}
        G_{\vtheta}(u^{(i)})(y^{(i)}_j) \right. &~,  \left.  \nabla_{\vtheta} G_{\vtheta}(u^{(i')})(y^{(i')}_{j'})  \right\rangle \\
        & = \sum_{k,k'=1}^K g_k\left(\vtheta_g; y^{(i)}_j\right) g_{k'}\left(\vtheta_g; y^{(i')}_{j'} \right) \left\langle \nabla_{\vtheta_f} f_k \left(\vtheta_f; u^{(i)}\right)~,  \nabla_{\vtheta_f} f_{k'} \left(\vtheta_f; u^{(i')}\right) \right\rangle \\
        & \phantom{=} + \sum_{k,k'=1}^K f_k \left(\vtheta_f; u^{(i)}\right) f_{k'} \left(\vtheta_f; u^{(i')}\right) \left\langle \nabla_{\vtheta_g} g_k\left(\vtheta_g; y^{(i)}_j\right)~, \nabla_{\vtheta_g} g_{k'}\left(\vtheta_g; y^{(i')}_{j'}\right) \right\rangle \\
        & = \sum_{k=1}^K \underbrace{g_k\left(\vtheta_g; y^{(i)}_j\right) g_{k}\left(\vtheta_g; y^{(i')}_{j'} \right)}_{T^{(1)}_k} \left\langle \nabla_{\vtheta_f} f_k \left(\vtheta_f; u^{(i)}\right)~,  \nabla_{\vtheta_f} f_{k} \left(\vtheta_f; u^{(i')}\right) \right\rangle \\
        & \phantom{=} + \sum_{k=1}^K \underbrace{f_k \left(\vtheta_f; u^{(i)}\right) f_{k} \left(\vtheta_f; u^{(i')}\right)}_{T^{(2)}_k} \left\langle \nabla_{\vtheta_g} g_k\left(\vtheta_g; y^{(i)}_j\right)~, \nabla_{\vtheta_g} g_{k}\left(\vtheta_g; y^{(i')}_{j'}\right) \right\rangle \\
        & \phantom{=} + \sum_{\substack{k,k'=1\\k \neq k'}}^K \underbrace{g_k\left(\vtheta_g; y^{(i)}_j\right) g_{k'}\left(\vtheta_g; y^{(i')}_{j'} \right)}_{T^{(3)}_{k,k'}} \left\langle \nabla_{\vtheta_f} f_k \left(\vtheta_f; u^{(i)}\right)~,  \nabla_{\vtheta_f} f_{k'} \left(\vtheta_f; u^{(i')}\right) \right\rangle \\
        & \phantom{=}  + \sum_{\substack{k,k'=1\\k \neq k'}}^K \underbrace{f_k \left(\vtheta_f; u^{(i)}\right) f_{k'} \left(\vtheta_f; u^{(i')}\right)}_{T^{(4)}_{k,k'}} \left\langle \nabla_{\vtheta_g} g_k\left(\vtheta_g; y^{(i)}_j\right)~, \nabla_{\vtheta_g} g_{k'}\left(\vtheta_g; y^{(i')}_{j'}\right) \right\rangle~. 
    \end{aligned}
    \label{eq:T3KKpNTK}
\end{align}
\NTKPD*
\begin{proof}
    The proof follows as a direct consequence of Proposition~\ref{prop:E_Tkkprime_NTK} together with Propositions~\ref{prop:quadraticFormNTK} and \ref{prop:NTKPosDef_DeepONet}
    \label{theo:NTKPosDef}
\end{proof}

\begin{prop}\label{prop:E_Tkkprime_NTK}
With the branch and trunk net weights initialized using standard initialization techniques and the last layer of branch layer initialized according to Assumption~\ref{asmp:smoothinit}, we have
    \begin{equation}
        \E[ T^{(3)}_{k,k'} | \vtheta_{\bar{g}}, \vtheta_{\bar{g}}] = 0~, \quad \E[ T^{(4)}_{k,k'} | \vtheta_{\bar{f}}, \vtheta_{\bar{f}}] = 0~,\quad k,k' \in [K]~.     
    \end{equation}
    where $T^{(3)}_{k,k'}$ is defined in \eqref{eq:T3KKpNTK}
\end{prop}
\proof
As noted in Assumption~\ref{asmp:smoothinit}, the last layer weights for the branch and trunk nets are initialized as zero mean Gaussians, i.e., $w_{k,h}^{(f)}, w_{k,h'}^{(g)} \sim \cN(0,\frac{1}{m K})$ for $k \in [K], h \in [m_f], h' \in [m_g]$, similar to the other layers. 
% Based on this initialization, conditioned on 
% the weights $(\vtheta_{\bar{g}}, \vtheta_{\bar{g}})$ till the prefinal layer, taking conditional expectation w.r.t.~the last layer weights,
% we have
% \begin{equation}
% \E[ T^{(3)}_{k,k'} | \vtheta_{\bar{g}}, \vtheta_{\bar{g}}] = 0~, \quad \E[ T^{(4)}_{k,k'} | \vtheta_{\bar{g}}, \vtheta_{\bar{g}}] = 0~,\quad k,k' \in [K]~.     
% \end{equation}
Now, 
\begin{align}
    \begin{aligned}
        T^{(3)}_{k,k'} & = g_k\left(\vtheta_g; y^{(i)}_j\right) g_{k'}\left(\vtheta_g; y^{(i')}_{j'} \right) \\
        & = \left(\sum_{h'=1}^{m_g} w_{k,h'}^{(g)} \bar{g}_{h'} \left(\vtheta_{\bar{g}}; y^{(i)}_j \right) \right) \left(\sum_{\tilde{h}'=1}^{m_g} w_{k',\tilde{h}'}^{(g)} \bar{g}_{\tilde{h}'} \left(\vtheta_{\bar{g}}; y^{(i')}_{j'} \right) \right) \\
        & = \sum_{h',\tilde{h}'=1}^{m_g}  w_{k,h'}^{(g)} w_{k',\tilde{h}'}^{(g)} \bar{g}_{h'} \left(\vtheta_{\bar{g}}; y^{(i)}_j \right) \bar{g}_{\tilde{h}'} \left(\vtheta_{\bar{g}}; y^{(i')}_{j'} \right)~,
    \end{aligned}
\end{align}
which in turn implies 
\begin{align}
    \begin{aligned}
        \E[ T^{(3)}_{k,k'} | \vtheta_{\bar{g}}, \vtheta_{\bar{g}}] & 
        = \sum_{h',\tilde{h}'=1}^{m_g}  \E[w_{k,h'}^{(g)} w_{k',\tilde{h}'}^{(g)}] \bar{g}_{h'} \left(\vtheta_{\bar{g}}; y^{(i)}_j \right) \bar{g}_{\tilde{h}'} \left(\vtheta_{\bar{g}}; y^{(i')}_{j'} \right) \\
        & \overset{(a)}{=} \sum_{h',\tilde{h}'=1}^{m_g}  \E[w_{k,h'}^{(g)}] \E[w_{k',\tilde{h}'}^{(g)}] \bar{g}_{h'} \left(\vtheta_{\bar{g}}; y^{(i)}_j \right) \bar{g}_{\tilde{h}'} \left(\vtheta_{\bar{g}}; y^{(i')}_{j'} \right)\\
        & = 0~,
    \end{aligned}
\end{align}
where (a) follows since $w_{k,h'}^{(g)}$ and $w_{k',\tilde{h}'}^{(g)}$ are independent. The analysis for $T^{(4)}_{k,k'}$ is similar. This completes the proof. \qed

% Further, one can get a high probability bound by using Hoeffding.

\begin{prop}\label{prop:E_Tkkprime_NTK_highprob}
With the branch and trunk net weights initialized using standard initialization techniques and the last layer of branch layer initialized according to Assumption~\ref{asmp:smoothinit}, we have for any $k,k' \in [K], k \neq k'$ 
    \begin{align}
        \P\left[ \left|\sum_{k\neq k'} T^{(3)}_{k,k'} \right| \leq \epsilon \mid \bar{\g} \right] & \geq 1 - 2 \exp \left(- \frac{m^2 \epsilon^2}{\|\bar{\g}\|_2^4} \right)~, \\
      \P\left[ \left|\sum_{k\neq k'} T^{(4)}_{k,k'} \right| \leq \epsilon \mid \bar{\f} \right] & \geq 1 - 2 \exp\left(- \frac{m^2 \epsilon^2}{\|\bar{\f}\|_2^4} \right) ~,
    \end{align}
    where $T^{(3)}_{k,k'}, T^{(4)}_{k,k'}$ are as defined in \eqref{eq:T3KKpNTK}. 
\end{prop}
\proof For $k \neq k'$, since
\begin{align*}
T^{(3)}_{k,k'} & = \sum_{h',\tilde{h}'=1}^{m_g}  w_{k,h'}^{(g)} w_{k',\tilde{h}'}^{(g)} \bar{g}_{h'} \left(\vtheta_{\bar{g}}; y^{(i)}_j \right) \bar{g}_{\tilde{h}'} \left(\vtheta_{\bar{g}}; y^{(i')}_{j'} \right)~,
\end{align*}
we can view $T^{(3)}_{k,k'}$ as a linear form  $\langle X, \a \rangle$ of $m_g^2$ independent Gaussian random variables $X_{h,h'} = w_{k,h'}^{(g)} w_{k',\tilde{h}'}^{(g)}, h,h' \in [m_g]$ with zero mean and variance $\frac{1}{K^2 m^2}$, and where $\a = \bar{\g} \otimes \bar{\g}$, the Kronecker product of $\bar{\g}$ with itself. Then, $\sum_{k\neq k'} T^{(3)}_{k,k'}$ can also be written as a linear form  $\langle \bar{X}, \bar{\a} \rangle$  of $k(k-1) m_g^2$ independent Gaussian random variables $X_{h,h',k,k'} = w_{k,h'}^{(g)} w_{k',\tilde{h}'}^{(g)}, h,h' \in [m_g], k,k' \in [K], k \neq k'$ with zero mean and variance $\frac{1}{k^2 m^2}$, and where $\bar{\a}$ is $k(k-1)$ times concatenation of $\a = \bar{\g} \otimes \bar{\g}$. Then, by Hoeffding's inequality, we have 
\begin{align*}
   \P\left[ \left|\sum_{k\neq k'} T^{(3)}_{k,k'} \right| > \epsilon \mid \bar{\g} \right]  =  \P\left[ \left| \langle \bar{X}, \bar{\a} \rangle \right| > \epsilon \mid \bar{\g} \right]  
   & \leq 2 \exp\left( - \frac{\epsilon^2}{\frac{1}{K^2 m^2} \| \bar{\a} \|_2^2 } \right) \\
   & = 2 \exp\left( - \frac{K^2 m^2 \epsilon^2}{ K(K-1) \| \a \|_2^2 } \right) \\
   & \leq 2 \exp\left( - \frac{ m^2 \epsilon^2}{ \| \bar{\g} \|_2^4 } \right)~,
\end{align*}
where we have used $\| \a \|_2 = \| \bar{\g} \otimes \bar{\g} \|_2 = \| \bar{\g} \|_2^2$. Switching the order of inequalities gives the desired result. 
The proof for $T^{(4)}_{k,k'}$ is essentially the same, but using $\bar{\f}$. \qed

In particular, choosing $\epsilon = \frac{1}{\sqrt{m}}$, we have 
   \begin{align}
        \P\left[ \left|\sum_{k\neq k'} T^{(3)}_{k,k'} \right| \leq \frac{1}{\sqrt{m}} \mid \bar{\g} \right] & \geq 1 - 2 \exp \left(- \frac{m}{\|\bar{\g}\|_2^4} \right)~, \\
      \P\left[ \left|\sum_{k\neq k'} T^{(4)}_{k,k'} \right| \leq \frac{1}{\sqrt{m}} \mid \bar{\f} \right] & \geq 1 - 2 \exp\left(- \frac{m }{\|\bar{\f}\|_2^4} \right) ~.
    \end{align}
In other words, the contribution from the cross-terms are smaller than $\frac{1}{\sqrt{m}}$ with high probability. 

\begin{prop}\label{prop:quadraticFormNTK}
    Given that the terms $T^{(3)}_{k,k'}$ and $T^{(4)}_{k,k'}$ can be suitably bounded close to zero, we have for any arbitrary block unit vector $\aalpha$ 
\begin{equation}
    \aalpha^T \gK(\vtheta) \aalpha \geq \lambda_{0,f} \sum_{k=1}^K \left\| \aalpha \odot g_k(\vtheta_g; \bfy^{(\cdot)}_{\cdot}) \right\|_2^2  + \lambda_{0,g} \sum_{k=1}^K \left\| \aalpha \odot \left(\1_p \otimes f_k(\vtheta_f; \bfu^{(\cdot)} \right) \right\|_2^2~.
    \label{eq:alphaT_K_alpha_lb}
\end{equation}
where $\1_q$ denotes the $q$-dimensional vector of all entries equal to one.
\end{prop}
\proof
Focusing on a quadratic form of $\gK(\vtheta)$, and ignoring the $T^{(3)}, T^{(4)}_{k,k'}$ terms, for any arbitrary block unit vector $\aalpha$, we have 
% \abcomment{notation mess: $k, K$ as last layer index, and $K$ as kernel}
\begin{align*}
\aalpha^T \gK(\vtheta) \aalpha &= \sum_{(i,j), (i',j')} \alpha_{i,j} \alpha_{i',j'} \left\langle  \nabla_{\vtheta}
G_{\vtheta}(u^{(i)})(y^{(i)}_j) \right. ~,  \left.  \nabla_{\vtheta} G_{\vtheta}(u^{(i')})(y^{(i')}_{j'})  \right\rangle \\
& = \sum_{(i,j), (i',j')} \alpha_{i,j} \alpha_{i',j'} 
\sum_{k=1}^K g_k\left(\vtheta_g; y^{(i)}_j\right) g_{k}\left(\vtheta_g; y^{(i')}_{j'} \right) \left\langle \nabla_{\vtheta_f} f_k \left(\vtheta_f; u^{(i)}\right)~,  \nabla_{\vtheta_f} f_{k} \left(\vtheta_f; u^{(i')}\right) \right\rangle \\
& \phantom{=} + \sum_{(i,j), (i',j')} \alpha_{i,j} \alpha_{i',j'} 
\sum_{k=1}^K f_k \left(\vtheta_f; u^{(i)}\right) f_{k'} \left(\vtheta_f; u^{(i')}\right) \left\langle \nabla_
{\vtheta_g} g_k\left(\vtheta_g; y^{(i)}_j\right)~, \nabla_{\vtheta_g} g_{k}\left(\vtheta_g; y^{(i')}_{j'}\right) \right\rangle \\
& = \sum_{k=1}^K \sum_{(i,j), (i',j')} \alpha_{i,j} \alpha_{i',j'} 
 g_k\left(\vtheta_g; y^{(i)}_j\right) g_{k}\left(\vtheta_g; y^{(i')}_{j'} \right) \left\langle \nabla_{\vtheta} f_k \left(\vtheta_f; u^{(i)}\right)~,  \nabla_{\vtheta} f_{k} \left(\vtheta_f; u^{(i')}\right) \right\rangle \\
& \phantom{=} + \sum_{k=1}^K  \sum_{(i,j), (i',j')} \alpha_{i,j} \alpha_{i',j'} 
f_k \left(\vtheta_f; u^{(i)}\right) f_{k} \left(\vtheta_f; u^{(i')}\right) \left\langle \nabla_{\vtheta} g_k\left(\vtheta_g; y^{(i)}_j\right)~, \nabla_{\vtheta} g_{k}\left(\vtheta_g; y^{(i')}_{j'}\right) \right\rangle \\
& = \sum_{k=1}^K   \sum_{(j,j')} \sum_{(i,i')}  \left( \alpha_{i,j} g_k\left(\vtheta_g; y^{(i)}_j\right) \right) \left( \alpha_{i',j'} g_{k}\left(\vtheta_g; y^{(i')}_{j'} \right)  \right) \left\langle   \nabla_{\vtheta} f_k \left(\vtheta_f; u^{(i)}\right)~,  \nabla_{\vtheta} f_{k} \left(\vtheta_f; u^{(i')}\right) \right\rangle \\
 & \phantom{=} + \sum_{k=1}^K \sum_{(i,j), (i',j')} \left(\alpha_{i,j} f_k \left(\vtheta_f; u^{(i)}\right)\right) \left( \alpha_{i',j'} f_{k} \left(\vtheta_f; u^{(i')}\right) \right) \left\langle  \nabla_{\vtheta} g_k\left(\vtheta_g; y^{(i)}_j\right)~,  \nabla_{\vtheta} g_{k}\left(\vtheta_g; y^{(i')}_{j'}\right) \right\rangle \\
 & \geq \sum_{k=1}^K \lambda_{\min}( \gK_{f,k} \otimes \I_q) \left\| \aalpha \odot g_k(\vtheta_g; \bfy^{(\cdot)}_{\cdot}) \right\|_2^2 + \lambda_{\min}( \gK_{g,k}) \left\| \aalpha \odot \left(\1_q \otimes f_k(\vtheta_f; \bfu^{(\cdot)} \right) \right\|_2^2 \\
 & \geq  \lambda_{0,f} \sum_{k=1}^K \left\| \aalpha \odot g_k(\vtheta_g; \bfy^{(\cdot)}_{\cdot}) \right\|_2^2  + \lambda_{0,g} \sum_{k=1}^K \left\| \aalpha \odot \left(\1_q \otimes f_k(\vtheta_f; \bfu^{(\cdot)} \right) \right\|_2^2 ~,
\end{align*}
where $\I_q$ denotes the $q$-dimensional identity matrix since $\alpha_{i,j} g_k\left(\vtheta_g; y^{(i)}_j\right)$ varies with $j$ whereas the kernel $K_f$ does not; $\1_q$ is the $q$-dimensional all ones vector since for the $\alpha_{i,j} f_k (\vtheta_f; u^{(i)})$ terms, for a fixed $i$, $\alpha_{i,j}$ differs with $j$ but $f_k \left(\vtheta_f; u^{(i)}\right)$ stays the same; $\lambda_{\min}( \gK_{f,k} \geq \lambda_{0,f}$; and $\lambda_{\min}( \gK_{g,k}) \geq \lambda_{0,g}$. This completes the proof. \qed

Note that we require $\aalpha$ is a block unit vector with $\aalpha_{i,j}$ denoting the $j$-th position in the $i$-th
for convenience in dealing with the quadratic form above.
Given that $T^{(3)}, T^{(4)}_{k,k'}$ terms are close to 0 in expectation, as shown in Proposition~\ref{prop:E_Tkkprime_NTK}, we now need to show that the NTK $\gK(\vtheta)$ is positive definite. 
% Subsequently, we show that bounding these terms close to zero by Hoeffding helps establish NTK to be positive definite with high probability. 

\begin{prop}\label{prop:NTKPosDef_DeepONet}
    Given that the terms $T^{(3)}_{k,k'}$ and $T^{(4)}_{k,k'}$ can be suitably bounded close to zero by Proposition~\ref{prop:E_Tkkprime_NTK}, we have, for any arbitrary block unit vector $\aalpha$, and some $k \in [K]$,
    \begin{align}
        \left\| \aalpha \odot g_k(\vtheta_g; \bfy^{(\cdot)}_{\cdot}) \right\|_2^2 \geq c_1 > 0~, \qquad \text{or} \qquad \left\| \aalpha \odot \left(\1_p \otimes f_k(\vtheta_f; \bfu^{(\cdot)} \right) \right\|_2^2 \geq c_2 > 0~,
    \end{align}
where $\1_q$ denotes the $q$-dimensional vector of all entries equal to one.
\end{prop}
\proof
Now, for the first term, for some $k \in [K]$, making use of \eqref{eq:fkone}, we have
\begin{align*}
\alpha_{i,j} g_k(\vtheta_g, \bfy_j^{(i)}) & = \sum_{h'=1}^{m_g} w_{k,h'}^{(g)} \alpha_{i,j} \bar{g}_{h'} \left( \vtheta_{\bar{g}} ; y^{(i)}_j \right) = \left\langle w_{k,\cdot}^{(g)} , \alpha_{i,j} \bar{g}_{\cdot} \left( \vtheta_{\bar{g}} ; y^{(i)}_j \right) \right\rangle~.
\end{align*}
Since the trunk net is a ReLU network, following the argument in Lemma 7.1 in \citet{allen-zhu_convergence_2019}, with probability at least $1 - O(q e^{-\Omega(m/4L)})$, for all $(i,j)$ we have $\left\| \bar{g}_{\cdot} \left( \vtheta_{\bar{g}} ; y^{(i)}_j \right) \right\|_2 \geq 1/2$. Recalling that $w_{k,h'}^{(g)} \sim \cN(0, \frac{1}{K})$, taking expectation over the randomness of $w_{k,h'}^{(g)}$, we have 
\begin{align*}
\E \left\| \aalpha \odot g_k(\vtheta_g; \bfy^{(\cdot)}_{\cdot}) \right\|_2^2 & = \sum_{(i,j)} \E \left\langle w_{k,\cdot}^{(g)} , \alpha_{i,j} \bar{g}_{\cdot} \left( \vtheta_{\bar{g}} ; y^{(i)}_j \right) \right\rangle^2 \\
& = \sum_{(i,j)} \left\langle \E[(w_{k,\cdot}^{(g)})^2] , \alpha_{i,j}^2 \bar{g}_{\cdot}^2 \left( \vtheta_{\bar{g}} ; y^{(i)}_j \right) \right\rangle \\
& = \sum_{(i,j)} \frac{\alpha_{i,j}^2}{K} \left\|   \bar{g}_{\cdot}^2 \left( \vtheta_{\bar{g}} ; y^{(i)}_j \right) \right\|_2^2 \\
& \geq \frac{1}{2K} \| \aalpha \|_2^2 = \frac{1}{2K}~.
\end{align*}
Hence, we have
\begin{align*}
 \lambda_{0,f} \E \sum_{k=1}^K \left\| \aalpha \odot g_k(\vtheta_g; \bfy^{(\cdot)}_{\cdot}) \right\|_2^2 \geq \frac{1}{2} \lambda_{0,f}~,
\end{align*}
and, with a similar argument 
\begin{align*}
\lambda_{0,g} \E \sum_{k=1}^K \left\| \aalpha \odot \left(\1_p \otimes f_k(\vtheta_f; \bfu^{(\cdot)} \right) \right\|_2^2 \geq \frac{1}{2} \lambda_{0,g}~.
\end{align*}
As a result, we have
\begin{align}
\aalpha^T \E \left[\gK(\vtheta) \right] \aalpha & \geq \frac{ \lambda_{0,f} + \lambda_{0,g}}{2} > 0~.    
\end{align}
The high probability version of the result can be obtained by applying Hoeffding (for cross terms) and Bernstein (for square terms) bounds on $\left\langle w_{k,\cdot}^{(g)} , \alpha_{i,j} \bar{g}_{\cdot} \left( \vtheta_{\bar{g}} ; y^{(i)}_j \right) \right\rangle^2$. That completes the analysis. \qed

\subsection{Experimental Details}\label{appdx:Experiments}

For the optimizer we choose \texttt{Adam} \citet{kingma2014adam} with an adaptive learning rate schedule initialized at a learning rate $\eta_0=10^{-3}$. %\abcomment{cite}. 
In order to generate training data for all three examples, we sample the input, denoted by $u(x)$, from a zero mean Gaussian process (GP) on a grid $\{x_l\}_{l=1}^m \in [0, 1]$ and generate outputs corresponding to each sampled function by solving the ODE/PDE (see \citet{wang_learning_2021,lu20201DeepONet} for a detailed discussion on data generation). For end-to-end training we use the deep learning framework JAX \citet{jax2018github} and build our code on top of \citet{wang_learning_2021} for Diffusion-Reaction and Antiderivative operators and we develop our own for the Burger's equation. We now briefly outline the problems below along with the specifics of the training process for each of them.
% \abcomment{what's the intended flow -- we will discuss the results as well after describing each problem, right?}
\subsubsection{Antiderivative Operator}\label{subsec:Antiderivative_Experiments}
The antiderivative (or simply the integral) operator corresponds to a linear operator defined explicitly by a linear ODE (initial value problem) in the unknown function $v(x)\in\mathcal{V}$, given the input $u(x)\in \mathcal{U}$, and the constant $v(0)$ for mathematical well-posedness, i.e.
\begin{equation}
    \frac{\rd v(x)}{d x} = u(x), \quad x \in[0,1] \quad \text{s.t.} \quad v(0) = 0.
\end{equation}
We learn the operator mapping $u(x)$ to its corresponding integral $v(x) = G_{\vtheta}(u)(x)$ for all $x\in(0, 1]$. For generating the training data, we sample the input functions from a univariate Gaussian process as outlined above and the output points randomly on the interval $[0, 1]$ and choose $n_B = 10000$ for our empirical results
% \abcomment{so, we are sampling functions from a Gaussian process (GP) ... lets just say that}
% \begin{equation}
%     k_{l}\left(x_{1}, x_{2}\right)=\exp \left(-\left\|x_{1}-x_{2}\right\|^{2} / 2 l^{2}\right).
%     \label{eq:Covariance_kernel_GRF}
% \end{equation}
% \abcomment{last bit unclear, seems there are two things going: generating the training data, which gets $s(x)$ from a ODE solver, and training the deeponet, is that based on JAX}
% (\url{https://github.com/google/jax/blob/main/jax/experimental/ode.py}). 
\subsubsection{Diffusion-Reaction PDE}
In this example we learn the operator mapping the input forcing function $u(x)$ to the output $v(x,t)$ for the nonlinear Diffusion-Reaction PDE given by
\begin{equation}
    \frac{\partial v}{\partial t}=D \frac{\partial^{2} v}{\partial x^{2}}
    +
    k v^{2} + u(x), \quad(x, t) \in(0,1] \times(0,1] \quad \text{s.t.}\quad \begin{cases}
    v(0,x)=0\\
    v(t,0)=0\\
    v(t,1)=0
    \end{cases}
    \label{eq:PDE_DiffusionReaction}
\end{equation}
where $D=0.01$ and $k=0.01$ are constants denoting the diffusivity and reaction rate respectively. Note that in this case we are learning the operator $v(x,t) = G_{\vtheta}(u)(x, t)$. For each sampled input, the PDE is solved using a backward finite-difference solver on a grid ($x,t$) of size ($150\times 120$). For training, the number of input sensors is fixed at $m=120$. The number of input samples ($n$) is chosen to be $5000$ and $n_B = 10000$.

\subsubsection{Burger's Equation}\label{subsec:Burgers_Experiments}
Finally, we look at the Burger's equation benchmark similar to the one investigated in \citet{li_fourier_2021} with the distinction that we learn a mapping from the initial condition $v(x, 0) = u(x)$ to the solution $v(x,t)$ for $(x,t)\in[0,1]\times (0,1]$
\begin{equation}
    \begin{aligned}
        & \del{v}{t}
        + v \del{v}{x}
        - 
        \nu \ddel{v}{x} = 0, \quad(x, t) \in(0,1) \times(0,1] \\
        & \begin{cases}
        v(x, 0)=u(x), \quad x \in(0,1) \\
        v(1, t) = v(0, t)\quad t \in (0,1)
        \end{cases}
    \end{aligned}
\label{eq:BurgersEquation_PDE}
\end{equation}
We generate the training data using a stiff PDE integrator \texttt{chebfun} \citet{driscoll2014chebfun} on a grid resolution of $(501, 501)$ and $p=200$ training points sampled randomly on the solution grid.
% \subsubsection{Results}
% We next summarize the results for all the experiments. The results make it plain that wider DeepONets based on over-parameterization lead to overall faster convergence during the training. The results for smooth activations  which complement the analysis in \Secref{sec:optimization} are summarized in \Figref{fig:SeLU_Loss} and the ones for ReLU activations are summarized in \Figref{fig:ReLU_Loss}. The training data is generated using a stiff PDE integrator in \texttt{chebfun} \citet{driscoll2014chebfun}.  
