# Supplementary material for: Optimization for Neural Operators can Benefit from Width
Source: arXiv:2502.00705 source file (2025-02-02)
Supplement: Supplementary file 2 [file holder.tex]

\subsection{Non-empty Restricted Set $Q^t_{\kappa}$ for DONs}

First, recall our definition of the $Q^t_{\kappa}$ set for DONs:
\qset*
We show that $Q^t_{\kappa}$ is non-empty.
\PropQtk*
\proof 
From the definition of $Q^t_{\kappa}$, $\vtheta'\in Q^t_{\kappa}$ needs to satisfy three conditions which we refer to as the cosine similarity condition, average condition, and output condition, for convenience:
\begin{align*}
|\cos(\vtheta' - \vtheta_t, \nabla_{\vtheta} \bar{G}_{\vtheta_t})| & \geq \kappa \quad \text{(cosine similarity condition)}~,\\
(\vtheta'_f-\vtheta_{f,t})^\top\left(\frac{1}{n} \sum_{i=1}^n \frac{1}{q_i} \sum_{j=1}^{q_i} \ell'_{i,j} \sum_{k=1}^K \nabla_{\vtheta_{f}} f_k^{(i)} \nabla_{\vtheta_{g}} g_{k,j}^{(i)~\top}\right)(\vtheta'_g-\vtheta_{g,t})  &\geq 0\quad \text{(average condition)}~,\\
(\vtheta'_f-\vtheta_{f,t})^\top\left( \sum_{k=1}^K \nabla_{\vtheta_{f}} f_k^{(i)} \nabla_{\vtheta_{g}} g_{k,j}^{(i)~\top}\right)(\vtheta'_g-\vtheta_{g,t})&\leq 0,\forall i\in[n],\forall j\in[q_i]
\quad \text{(output condition)}.
\end{align*}

We first notice that if $\vtheta'=\vtheta_t$, then the cosine similarity condition is not satisfied, and thus, $\vtheta_t\notin Q^t_{\kappa}$.

We also notice that the output condition is in reality a system of $q=\sum^n_{i=1}q_i$ quadratic inequalities, each one with $p_g+p_f$ variables, since $\vtheta'\in\R^{p_f+p_g}$ is the variable of interest.

Now, we prove that the $Q^t_{\kappa}$ set is non-empty. 
We simply construct a $\vtheta'={[{\vtheta'_f}^{\top}\;{\vtheta'_g}^{\top}]}^{\top} \in Q^t_{\kappa}\subset \R^{p_f+p_q}$ along with appropriate values for $\kappa$. Without loss of generality, we set $\vtheta_t\equiv \vzero_{p_f+p_g}$, i.e., $\vtheta_t$ to be the origin of the coordinate system (the zero vector of dimension $p_f+p_g$) and work with the unit vector $\bar{\g} = [\bar{\g}_f^{\top}\;\bar{\g}_g^{\top}]^{\top} =  \frac{\nabla_{\vtheta} \bar{G}_{\vtheta_t}}{\| \nabla_{\vtheta} \bar{G}_{\vtheta_t}\|_2}\in\R^{p_f+p_g}$, since the cosine similarity condition is invariant under different magnitudes. 
% \abcomment{the svd condition does, but we make it zero; so need a sentence showing why this is wlog}. 
%Further, we assume $\vtheta'=[{\vtheta'_f}^\top {\vtheta'_g}^\top]^\top \in \R^{p_f+p_g}$ also to be a unit vector. 
% \abdelete{Consider two singular bases $(\va_{h_1},\vb_{h_1}), (\va_{h_1},\vb_{h_1})$ with $\sigma_{h_1} \geq \sigma_{h_2}$ such that $\nabla_{\vtheta_f}$ has non-zero projections on $\va_{h_1}, \va_{h_2}$ and $\nabla_{\vtheta_g}$ has non-zero projections on $\vb_{h_1}, \vb_{h_2}$\abcomment{if time permits, handle the base case where this is violated: 1d case}.} 
Then, our problem reduces to feasibility of the following system of quadratic inequalities over $\vtheta'_f \in \R^{p_f}, \vtheta'_g \in \R^{p_g}$:
\begin{align*}
  \left( \langle \vtheta'_f , \bar{\g}_f \rangle + \langle \vtheta'_g , \bar{\g}_g \rangle \right)^2  & \geq \kappa^2 \quad \text{(cosine similarity condition)}~, \\
  (\vtheta'_f-\vtheta_{f,t})^\top\left(\frac{1}{n} \sum_{i=1}^n \frac{1}{q_i} \sum_{j=1}^{q_i} \ell'_{i,j} \sum_{k=1}^K \nabla_{\vtheta_{f}} f_k^{(i)} \nabla_{\vtheta_{g}} g_{k,j}^{(i)~\top}\right)(\vtheta'_g-\vtheta_{g,t})  &\geq 0\quad \text{(average condition)}~,\\
  \vtheta_f^{\prime\top}\left( \sum_{k=1}^K \nabla_{\vtheta_{f}} f_k^{(i)} \nabla_{\vtheta_{g}} g_{k,j}^{(i)~\top}\right)\vtheta'_g&\leq 0,\forall i\in[n],\forall j\in[q_i]
\quad \text{(output condition)}.
\end{align*}
%
%$\bar{\g}=[\bar{\g}_f^{\top}\;\bar{\g}_g^{\top}]^{\top} \in \R^{p_f+p_g}$ and $\vtheta' =[\vtheta'_f;\vtheta'_g] \in \R^{p_f+p_g}$ are unit vectors, and
%
%We will choose a suitable $\kappa \in (0,\frac{1}{2}]$. 
To build a first element in the set, without loss of generality, assume $\| \bar{\g}_f\|_2 \geq \| \bar{\g}_g \|_2$ (the case $\| \bar{\g}_f\|_2 \leq \| \bar{\g}_g \|_2$ is treated similarly) so that $\| \bar{\g}_f\|_2 \geq \frac{1}{\sqrt{2}}$. Then, set $\vtheta'_g = \mathbf{0}_{p_g}$ so that our feasibility conditions reduces to only having to satisfy $\langle \vtheta'_f, \bar{\g}_f \rangle^2 \geq \kappa^2$ for some suitably chosen $\kappa \in (0,1]$. Finally, set $\vtheta'_f = \frac{\bar{\g}_f}{\| \bar{\g}_f \|_2}$ so that 
\begin{align*}
\langle \vtheta'_f, \bar{\g}_f \rangle^2 = \left( \frac{\bar{\g}_f}{\| \bar{\g}_f \|_2} \bar{\g}_f  \right)^2 = \| \bar{\g}_f \|_2^2 \geq \frac{1}{2}~,
\end{align*}
so that the feasibility condition is satisfied for $\kappa \in (0,\frac{1}{\sqrt{2}}]$. This completes the proof. \qed
