# Supplementary material for: Optimization for Neural Operators can Benefit from Width
Source: arXiv:2502.00705 source file (2025-02-02)
Supplement: Supplementary file 3 [file learningDONFNO.tex]

\subsection{DON training tuple}
Each DON training data comprises of the tuple $\gD^{(i)}:=\left(\{u^{(i)}(x_r)\}_{r=1}^R,\, \{y^{(i)}_j\}_{j=1}^{q_i}, \{G(u^{(i)})(y^{(i)}_j)\}_{j=1}^{q_i}\right)$. The total training dataset comprises of all such training tuples $\gD = \{ \gD^{(i)}\}_{i=1}^n$.

\subsection{Motivation for FNOs}
FNOs are closely related to the notion of fundamental solutions. This allows us to write ${k_{l}:=}k\left(x, y, a(x), a(y) ; \vtheta_{\gF^{(l)}}\right) := k\left(x-y; \vtheta_{\gF^{(l)}}\right)$ \citep{li_fourier_2021}. Taking the Fourier Transform ($\mathscr{F}$) and applying the convolution theorem gives
$\left(\mathcal{K}^{(l)}(a ;  \vtheta_{\gF^{(l)}}) \alpha^{(l-1)}\right)(x)=
\mathscr{F}^{-1}\left(\mathscr{F}\left(k_l\right) \cdot \mathscr{F}\left(\alpha^{(l-1)}\right)\right)(x)$, $\forall x \in \gT$, $l\in [L]$.

This helps in parameterizing the \emph{kernel operator} $R^{(l)} = \mathscr{F}(k_l)$ directly in the Fourier space {and in simplified notation obtain}, 
$\left(\mathcal{K}^{(l)} \alpha^{({l-1})}\right)(x)
=\mathscr{F}^{-1}\left(R^{(l)} \cdot\left(\mathscr{F} \alpha^{({l-1})}\right)\right)(x)$, $\forall x \in \gT$, $l\in [L]$.

{Replacing this quantity back in~\eqref{eq:nonFnoLay},} 
following \citep{li_fourier_2021}, we define each Fourier block as follows
\begin{align}
    \alpha^{(l)}(x)
    =
    \phi\left(W^{(l)} \alpha^{(l-1)} 
    + 
    \mathscr{F}^{-1}\left(R^{(l)} \cdot \mathscr{F}\left(\alpha^{(l-1)}\right)\right)\right)(x), \quad x\in\gT, \quad l \in [L],
    \label{eq:ContinuousFNOBlocks}
\end{align}
where 
the Fourier transform of the input function $\alpha^{({l-1})}$ is $\mathscr{F}\alpha^{({l-1})}(\xi) := \int_{\gT} e^{-2\pi i <\xi ,y>} \alpha^{({l-1})}(y) dy$, $y\in \gT$.
{Notice that $R^{(l)}$ is defined by the set of unknown parameters $\vtheta_{\gF^{(l)}}$, whereas $\vtheta_{F^{(l)}}$ is defined by both the affine operator $W^{(l)}$ and parameters $\vtheta_{\gF^{(l)}}$.}
%
% \begin{remark}
% The input $a$, output $u$ and the intermediate functions $\alpha^{(l)}$, $l\in[L]$, in~\eqref{eq:ContinuousFNOBlocks} are all functions, {unlike the case of standard neural networks where they would be vectors.} \pcdelete{(like in standard neural networks).} \bscomment{maybe be a bit more precise on the what spaces these belong to}\pccomment{I agree -- at least the intermediate functions should be such that a Fourier transform exists (i.e., is well-defined)}\qed  
% \end{remark}
We now turn to the discrete version of \eqref{eq:ContinuousFNOBlocks} and the associated architecture.

{Since we have a discrete domain,} we employ the Discrete Fourier Transform (DFT). The entries of the ${m}\times {m}$ DFT kernel ($F$) can be written (up to a suitable scaling) as $F_{kj}:= e^{\frac{-2\pi i}{{m}}(k-1)(j-1)}$, where $k, j \in [{m}]$ which allows us to write its action on an input vector $\aalpha^{(l-1)}{\in\mathbb{R}^m}$ as
    \begin{equation}
        v_k := \sum_{j=1}^{{m}} F_{kj}\alpha^{(l-1)}_j = \alpha^{(l-1)}_j e^{\frac{-2\pi i}{{m}}(k-1)(j-1)},
    \end{equation}
where $i^2 = -1$.
